# Supplementary material for: ScaleNet: A Shallow Architecture for Scale Estimation
Source: arXiv:2112.04846 source file (2022-07-05)
Supplement: Supplementary file 1 [file 06_code.tex]

\section{Code}
\label{appendix_sec:code}
\begin{figure}[t]
 \vspace{0.15cm}
 \hspace{-0.19cm}
%  \centering
  \includegraphics[scale=0.35]{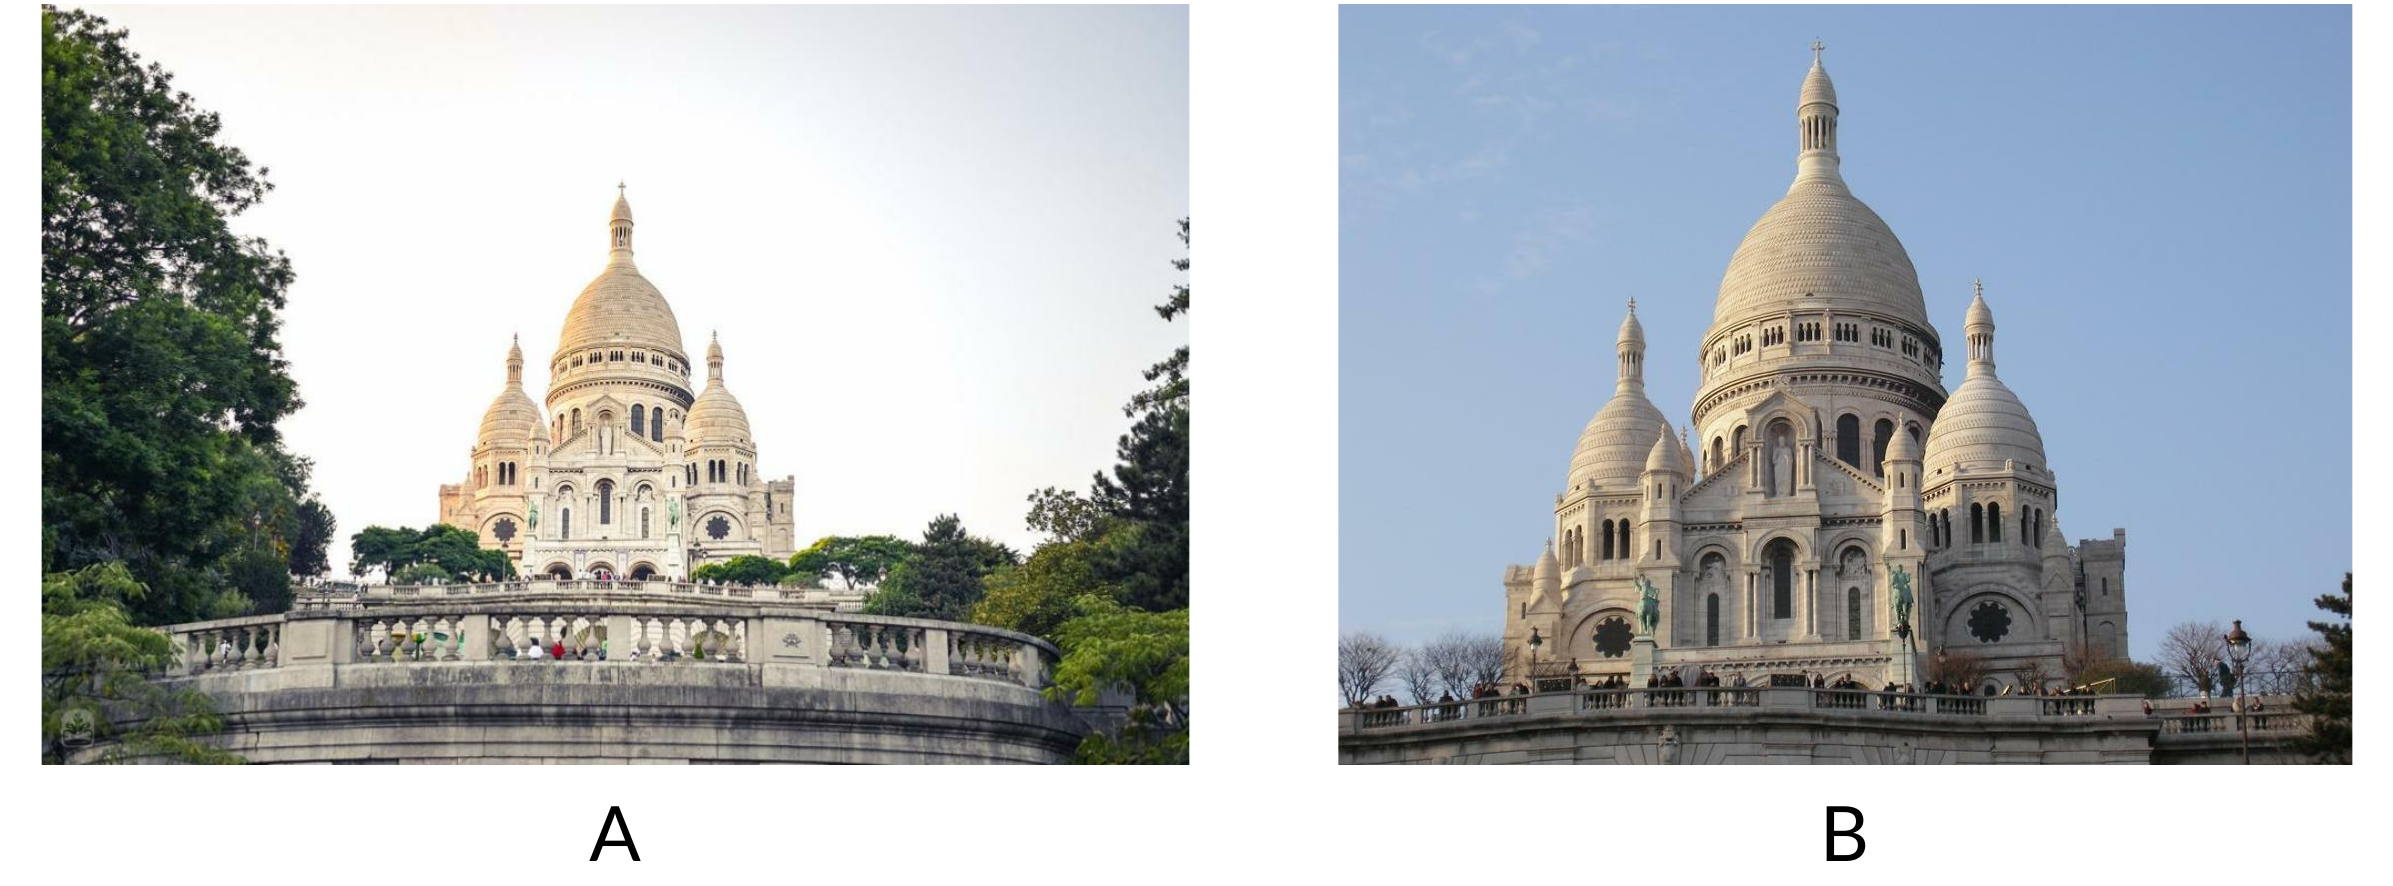}
    \caption{Example of the image pair contained within the \textit{code} folder. ScaleNet scale factor prediction for $A \rightarrow B$ and $A \leftarrow B$ is 1.85 and 0.54, respectively.}
    \label{appendix_fig:example_code}
\end{figure}
Along with the architecture details in section \ref{appendix_sec:implementation}, we also provide the code for ScaleNet with its trained weights. The code can be found in the \textit{code} folder. For running ScaleNet and computing the scale factor between two images, please run the python script \textit{run\_scalenet.py}. Change \textit{im1\_path} and \textit{im2\_path} arguments for testing ScaleNet with your own images. In figure \ref{appendix_fig:example_code}, we show the two images from  \textit{im\_test} folder. ScaleNet factor predicted for $A \rightarrow B$ and $A \leftarrow B$ is 1.85 and 0.54, respectively.
