# Supplementary material for: ScaleNet: A Shallow Architecture for Scale Estimation
Source: arXiv:2112.04846 source file (2022-07-05)
Supplement: Supplementary file 2 [file code_fig.tex]

\begin{figure}[t]
 \vspace{0.15cm}
 \hspace{-0.19cm}
%  \centering
  \includegraphics[scale=0.35]{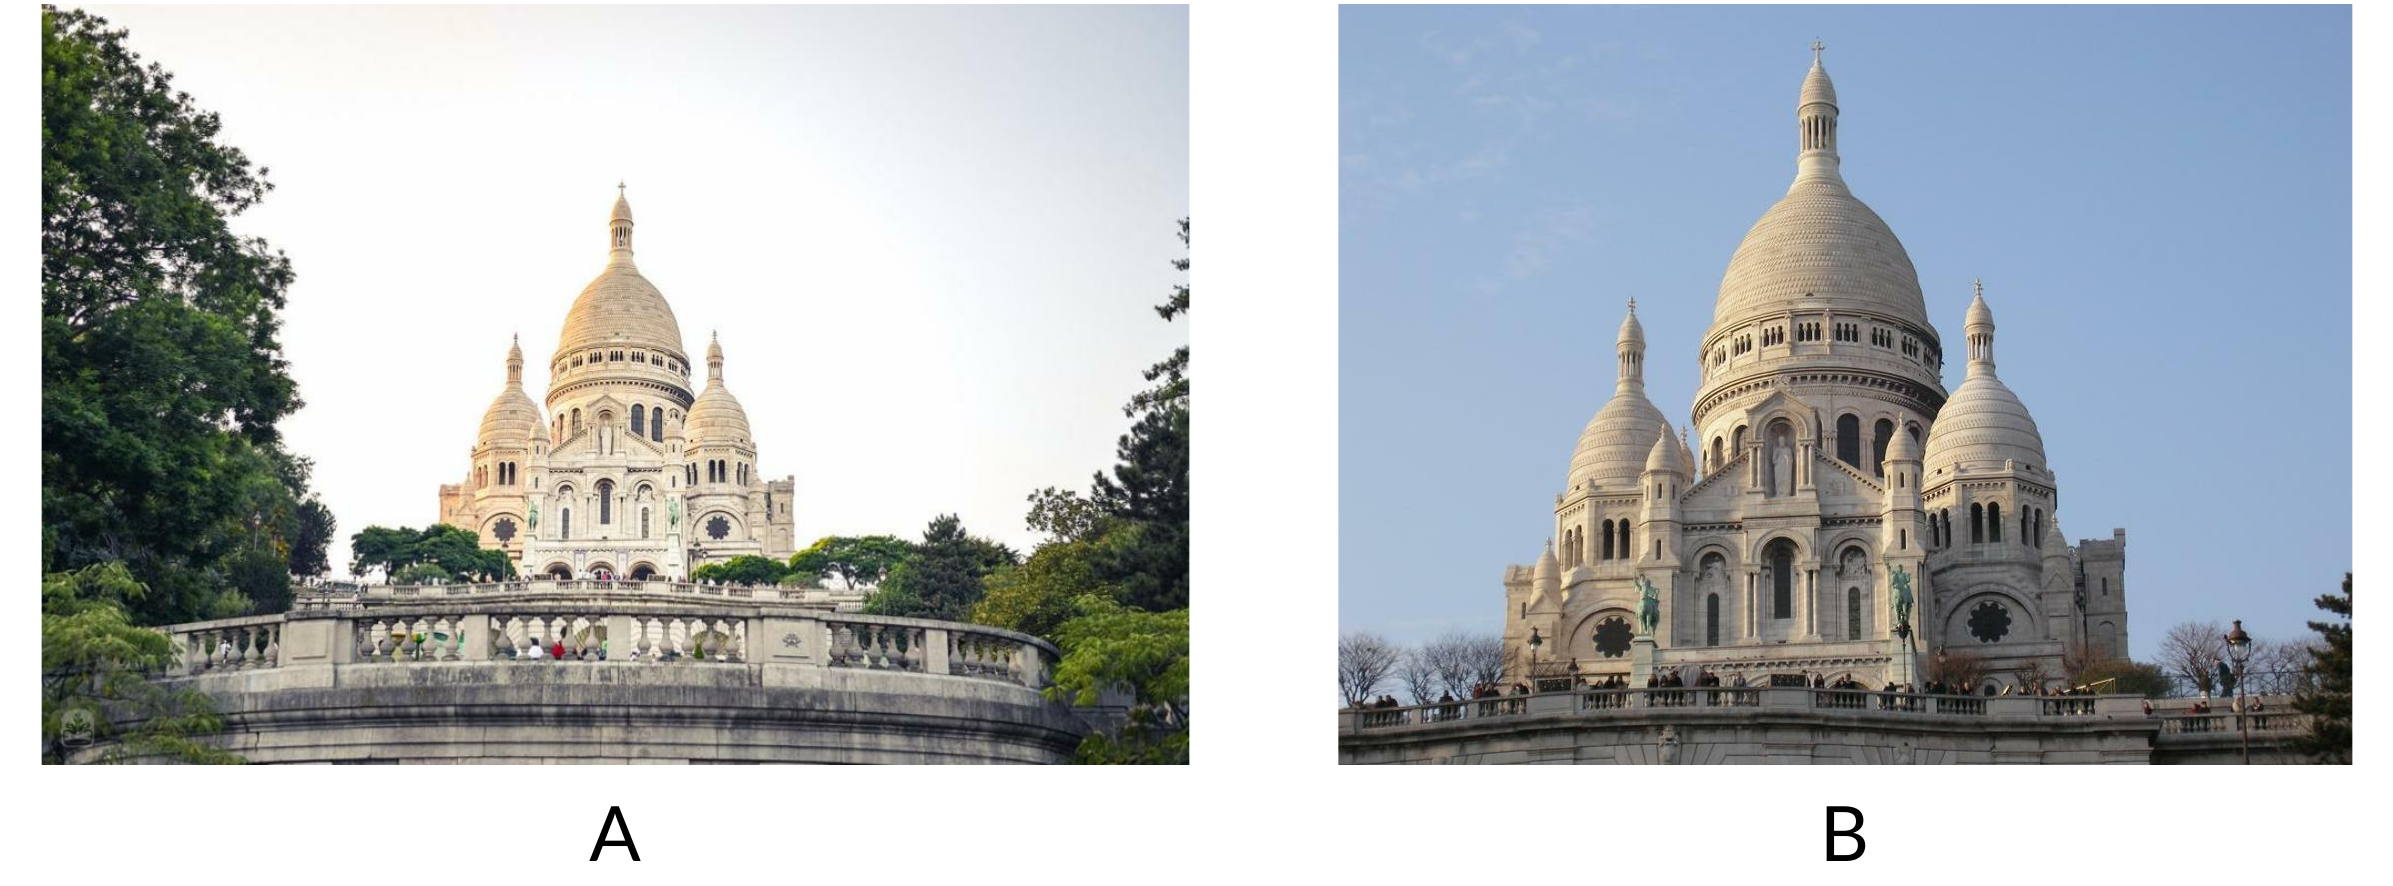}
    \caption{Example of the image pair contained within the \textit{code} folder. ScaleNet scale factor prediction for $A \rightarrow B$ and $A \leftarrow B$ is 1.85 and 0.54, respectively.}
    \label{appendix_fig:example_code}
\end{figure}
