# Supplementary material for: ScaleNet: A Shallow Architecture for Scale Estimation
Source: arXiv:2112.04846 source file (2022-07-05)
Supplement: Supplementary file 3 [file hist_dataset.tex]

\begin{figure}[t]
 \centering
  \includegraphics[scale=0.34]{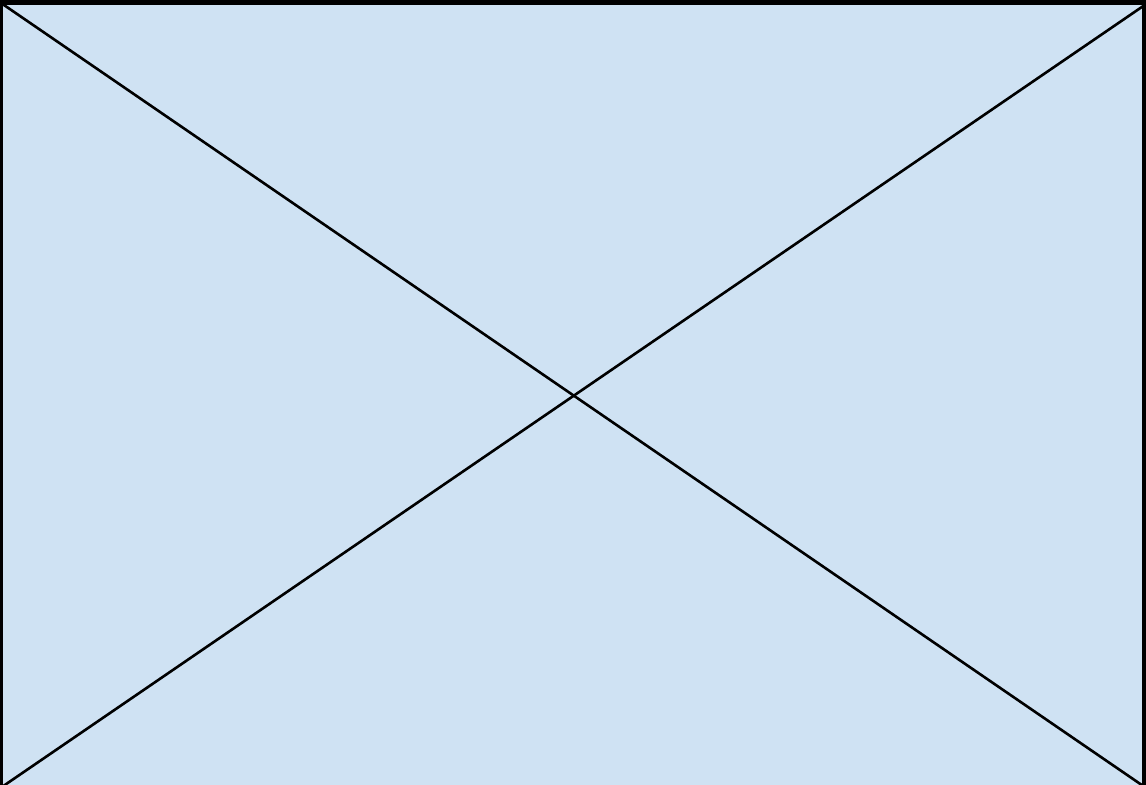}
    \caption{histogram.}
    \label{appendix_fig:dataset_hist}
\end{figure}
