# Supplementary material for: ScaleNet: A Shallow Architecture for Scale Estimation
Source: arXiv:2112.04846 source file (2022-07-05)
Supplement: Supplementary file 4 [file local_scalenet_example.tex]

\begin{figure}[]
% \vspace{-0.20cm}
 \centering
%  \hspace{-0.50cm}
  \includegraphics[scale=0.7]{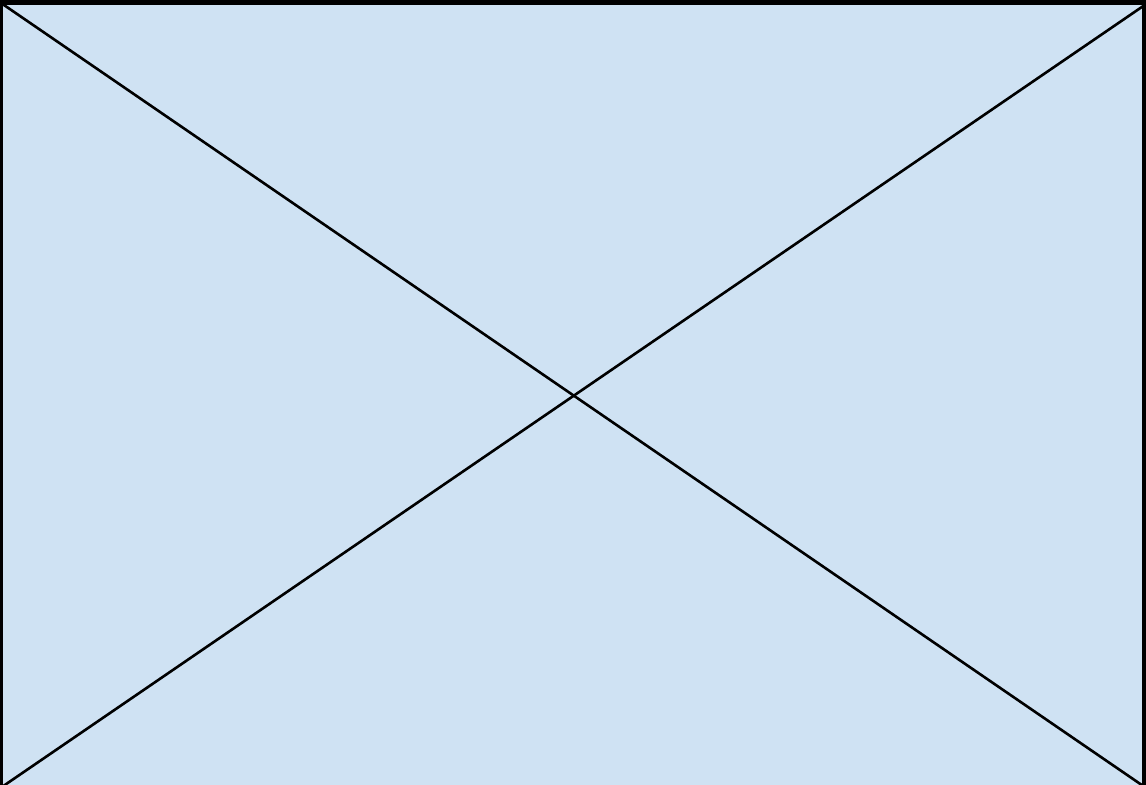}
    \caption{Example of local scale estimations on the \textit{v\_courses} sequence from HPatches. In contrast to global ScaleNet, Local-ScaleNet uses a CNN prediction block to output a dense scale map.}
    \label{appendix_fig:local_estimations}
    % \vspace{-0.3cm}
\end{figure}
