# Supplementary material for: ScaleNet: A Shallow Architecture for Scale Estimation
Source: arXiv:2112.04846 source file (2022-07-05)
Supplement: Supplementary file 5 [file architecture_blocks.tex]

\begin{table}[]
% \tiny
\footnotesize
\begin{center}
\begin{tabular}{c c c c }
% \hline \noalign{\smallskip}
% \cline{2-9} \noalign{\smallskip}
\multicolumn{4}{c}{\textbf{Feature Reduction Block}}\\
\hline \noalign{\smallskip}
Layer & Description & In & Out\\
\hline \noalign{\smallskip}
1 & Conv-Batch-ReLU & 1 x 512 x 15 x 15 &  1 x 256 x 13 x 13 \\
2 & Conv-Batch-ReLU & 1 x 256 x 13 x 13 &  1 x 128 x 11 x 11 \\
3 & Conv-Batch-ReLU & 1 x 128 x 11 x 11 &  1 x 64 x 9 x 9\\
4 & Conv-Batch-ReLU & 1 x 64 x 9 x 9 &  1 x 32 x 7 x 7\\
5 & Flatten & 1 x 32 x 7 x 7 &  1 x 1568 \\
\end{tabular}
\end{center}
\normalsize
\vspace{-0.30cm}
\caption{Feature reduction block after the correlation layers within ScaleNet architecture. The block process the correlation maps, $c_A$, $c_B$, and $c_{A-B}$, into lower resolution maps.}
\label{appendix_tab:scalenet_block1}
\end{table}

\begin{table}[]
% \tiny
\footnotesize
\begin{center}
\begin{tabular}{c c c c }
% \hline \noalign{\smallskip}
% \cline{2-9} \noalign{\smallskip}
\multicolumn{4}{c}{\textbf{Fully Connected Layers}}\\
\hline \noalign{\smallskip}
Layer & Description & In & Out\\
\hline \noalign{\smallskip}
1 & Conv-Batch-ReLU & 1 x 4704 &  1 x 2056 \\
2 & Conv-Batch-ReLU & 1 x 2056 &  1 x 1024 \\
3 & Conv-Batch-ReLU & 1 x 1024 &  1 x 512 \\
4 & Conv-Batch-ReLU & 1 x 512 &  1 x 256 \\
5 & Conv-Batch-ReLU & 1 x 256 &  1 x 128 \\
6 & Conv-Softmax & 1 x 128 &  1 x $L$ \\
\end{tabular}
\end{center}
\normalsize
\vspace{-0.30cm}
\caption{Description of the final fully connected layers within the ScaleNet architecture that compute the scale distribution from the flatten correlation maps.}
\label{appendix_tab:scalenet_block2}
\end{table}
