# Supplementary material for: ScaleNet: A Shallow Architecture for Scale Estimation
Source: arXiv:2112.04846 source file (2022-07-05)
Supplement: Supplementary file 6 [file local_architecture_blocks.tex]

\begin{table}[]
% \tiny
\footnotesize
\begin{center}
\begin{tabular}{c c c c }
% \hline \noalign{\smallskip}
% \cline{2-9} \noalign{\smallskip}
\multicolumn{4}{c}{\textbf{Local Feature Reduction Block}}\\
\hline \noalign{\smallskip}
Layer & Description & In & Out\\
\hline \noalign{\smallskip}
1 & Conv-Batch-ReLU & 1 x 512 x 15 x 15 &  1 x 256 x 15 x 15 \\
2 & Conv-Batch-ReLU & 1 x 256 x 15 x 15 &  1 x 128 x 15 x 15 \\
3 & Conv-Batch-ReLU & 1 x 128 x 15 x 15 &  1 x 64 x 15 x 15\\
4 & Conv-Batch-ReLU & 1 x 64 x 15 x 15 &  1 x 32 x 15 x 15\\
\end{tabular}
\end{center}
\normalsize
\vspace{-0.30cm}
\caption{Local feature reduction block within Local-ScaleNet architecture for $c_A$ and $c_{A-B}$ correlation maps.}
\label{appendix_tab:local_scalenet_block1}
\end{table}

\begin{table}[]
% \tiny
\footnotesize
\begin{center}
\begin{tabular}{c c c c }
% \hline \noalign{\smallskip}
% \cline{2-9} \noalign{\smallskip}
\multicolumn{4}{c}{\textbf{Dense Prediction Block}}\\
\hline \noalign{\smallskip}
Layer & Description & In & Out\\
\hline \noalign{\smallskip}
1 & Conv-Batch-ReLU & 1 x 64 x 15 x 15 &  1 x 32 x 15 x 15  \\
2 & Conv-Batch-ReLU & 1 x 32 x 15 x 15 &  1 x 16 x 15 x 15 \\
3 & Conv-Softmax & 1 x 16 x 15 x 15 &  1 x $L$ x 15 x 15 \\
\end{tabular}
\end{center}
\normalsize
\vspace{-0.30cm}
\caption{Last CNN block within the Local-ScaleNet architecture that computes the dense scale factor map.}
\label{appendix_tab:local_scalenet_block2}
\end{table}
